# Supplementary material for: A multiwavelength survey of HI-excess galaxies with surprisingly inefficient star formation
Source: arXiv:1801.06880 source file (2018-01-21)
Supplement: Supplementary file 1 [file Appendix.tex]

\section{Additional information}\label{Sec:Appendix}

This Section contains the comparison between Arecibo and GMRT global \HI\ profiles, and information on the environmental properties of the four \HI-excess galaxies (in Table \ref{table:appendix}).

%\topmargin2cm
%\textheight29cm
%\newpage
%\pagestyle{empty}
%\begin{figure*}
%\begin{picture}(600,600)(0,0)
%\graphpaper(-50,-100)(500,700)
%\put(-60,390){\framebox(290,140){}}
%\put(-20,475){\includegraphics[width=.22\textwidth]{Plots/SDSS_G20339.png}}
%\put(90,460){\includegraphics[width=.9\textwidth]{Plots/Collection_G20339.png}}
%\put(-20,320){\includegraphics[width=.22\textwidth]{Plots/SDSS_J1126.png}}
%\put(90,310){\includegraphics[width=.9\textwidth]{Plots/Collection_J1126.png}}
%\put(-20,175){\includegraphics[width=.22\textwidth]{Plots/SDSS_J1558.png}}
%\put(90,160){\includegraphics[width=.9\textwidth]{Plots/Collection_J1558.png}}
%\put(-20,20){\includegraphics[width=.22\textwidth]{Plots/SDSS_J1605.png}}
%\put(90,10){\includegraphics[width=.9\textwidth]{Plots/Collection_J1605.png}}
%\end{picture}
%\caption{Bla}
%\end{figure*}
